# Supplementary material for: Convex Iteration for Distance-Geometric Inverse Kinematics
Source: arXiv:2109.03374 source file (2022-07-06)
Supplement: Supplementary file 2 [file packages_supp.tex]

\let\proof\relax
\let\endproof\relax
\usepackage{amsmath} 
\usepackage{amssymb}
\usepackage{amsthm} % Needed for proper Theorem and Problem environments
% Use of \theoremstyle clashes with Cleverref, but we don't need remarks so it's OK.
%\let\proof\relax
%\theoremstyle{remark}
%\newtheorem*{remark}{Remark}
%\usepackage{times}

%\pdfinfo{
%   /Author (Homer Simpson)
%   /Title  (Robots: Our new overlords)
%   /CreationDate (D:20101201120000)
%   /Subject (Robots)
%   /Keywords (Robots;Overlords)
%}

%\usepackage[numbers,sort&compress]{natbib}
%\setlength{\bibsep}{4pt plus 0.5ex}


\usepackage{multicol}
\usepackage[bookmarks=true]{hyperref}

%Custom imports
\usepackage{xparse} 
\usepackage{amsfonts} 
\usepackage{dsfont}
\usepackage{graphicx}
\usepackage{url}
\usepackage{booktabs}
\usepackage[para]{threeparttable}
\usepackage{multirow}
\hypersetup{colorlinks,linkcolor={blue},citecolor={green},urlcolor={blue}}  

\usepackage{xcolor}
\usepackage{framed}
\usepackage{caption}
\usepackage{varwidth}
\usepackage{subcaption}
\usepackage[utf8]{inputenc}
\usepackage{pgfplots}
\usepackage{adjustbox}
\DeclareUnicodeCharacter{2212}{−}
\usepgfplotslibrary{groupplots,dateplot}
\usetikzlibrary{patterns,shapes.arrows}
\pgfplotsset{compat=newest}
\captionsetup{font=small}
\captionsetup[sub]{font=small}

% Messes up the supplement
%\usepackage{flushend}

%Useful for tables
\usepackage{pifont}
\newcommand{\cmark}{\ding{51}}%
\newcommand{\xmark}{\ding{55}}%

\usepackage[ruled,vlined]{algorithm2e}
\SetKwInOut{Parameters}{Parameters}
\newcommand*\Let[2]{\State #1 $\gets$ #2}
\usepackage{setspace}

%Cleverref stuff
\usepackage{cleveref}
%Spacing for non-mathmode definitions
\usepackage{xspace}

\colorlet{shadecolor}{gray!10}
\newenvironment{todo}[1]
   {\begin{shaded} {\color{red}\textbf{To-do}} (\textit{#1}).}
   {\end{shaded}}   
\newtheorem{problem}{Problem}
\newtheorem{assumption}{Assumption}
\newtheorem{theorem}{Theorem}
\newtheorem{proposition}{Proposition}
\newtheorem{corollary}{Corollary}
\newtheorem{definition}{Definition}
